# Supplementary material for: Evaluating the Robustness of Semantic Segmentation for Autonomous Driving against Real-World Adversarial Patch Attacks
Source: arXiv:2108.06179 source file (2021-08-13)
Supplement: Supplementary file 1 [file appendix.tex]

\appendix

\section{Loss functions for physical realizability} \label{s:physical_loss}
Classical adversarial examples (sometimes referred to ``digital" adversarial examples) rely on image-sized additive perturbations $r$, that require the optimization of a single loss function $\LOSS_{adv}$ (the adversarial loss). This loss function expresses, in the untargeted attack formulation, the distance of the network prediction corresponding to the adversarial image $x+r$ from the true label corresponding to the input image $x$.

Although this loss function is sufficient to optimize classical adversarial examples, these rely on the assumption that the attacker has full control on the digital representation of the image. This is difficult to obtain for safety-critical systems. 
Hence, adversarial examples should lay in the physical world and still maintain their fooling power when they enter the field of view of the camera providing the input image for the perception system.
Also, usually, a real-world perception system is composed of several different modules, including preprocessing functions, such as crop, resize, and other data augmentations techniques.

These factors explain the need for a more specialized adversarial loss function, which is based on universal perturbations \cite{2016arXiv161008401M} (to produce image-agnostic perturbations), and the EOT paradigm \cite{pmlr-v80-athalye18b} (to render the perturbation robust to transformations typical of the real world), as explained in the paper.

However, physical realizability is another important factor that has to be accounted for. In particular, it is likely that the printer used to print the adversarial perturbation is not able to print the entire continuous spectrum of colors. Hence, the non-printability score \cite{sharif_accessorize_2016} is introduced to take into account this effect. Assuming that a pixel $p$ of the patch $\delta$ is composed of an RGB triplet, the non-printability score $\LOSS_N$ is defined as 
\begin{equation}
    \LOSS_N(p)=\prod\limits_{c\in C}\|p-c\|
\end{equation}
\noindent where $C$ is the set of RGB triplets that compose the printable color palette of the printer. The non-printability score is then averaged for the totality of pixels in the perturbation, and should be low when the totality of the patch pixel colors is close to the printable ones.

Also, typical digital perturbations are very noisy, since there is very little correlation between adjacent pixels. This patterns in the real world are smoothed out by both the printing process, and the camera acquisition process (which introduces noise and blurring). This effect can be taken into account by considering another additional loss, the ``smoothness" loss, defined as
\begin{equation}
    \LOSS_S = \sum\limits_{i}\sum\limits_{j}[(\delta_{i+1, j} - \delta_{i, j})^2 + \delta_{i, j+1} - \delta_{i, j})^2]
\end{equation}
\noindent where $(i, j)$ are the 2D index of the adversarial perturbation. This additional loss function introduces correlation between adjacent pixels, and should help craft a more ``smooth" perturbation, without noisy patterns.

Summing these additional loss terms, the total loss function for physical realizable real-world adversarial examples is
\begin{equation}
    \LOSS = w_{adv} \LOSS_{adv} + w_{N} \LOSS_N + w_{S} \LOSS_S
\end{equation}
\noindent where $w_{adv}, w_N, w_S$ are the weights corresponding to each loss components. 

In practice, the adversarial loss (for the untargeted attack formulation) tends to increase in norm during the optimization. This increase masks the effect of the other losses during the advancement of the optimization. To make the weighting actually effective, the gradient of each loss is computed individually, it is normalized, and then averaged according to the weights. This total gradient is applied to advance the optimization, as in Equation \ref{e:opt}.

The experiments in Section \ref{s:exp} are performed with $w_{adv}=1, w_N=0, w_S=1$. Empirically, we noticed that the non-printability score is not needed for this kind of evaluation, while the smoothness loss is crucial for transferring to the real world.

\section{Projective transformation for scene-specific attack} \label{s:impl}
The scene-specific attack, as explained in Section \ref{s:method}, requires a projective transformation to precisely apply the patch onto the 2D attackable surface. 

With the CARLA simulator, it is possible to extract the pose (with respect to the World reference frame) of both the attackable surface and the camera.

Using 3D rototranslation in homogeneous formulation, it is possible to express the position of a 3D point on the attackable surface $p^S$ (initially expressed in the surface reference frame) in the camera reference frame. Given that $T_a^b$ is the roto-translation matrix from generic reference frame $a$ to $b$, expressed as composition of a rotation matrix $R_a^b$ and translation vector $t_a^b$,
\begin{equation}
    T_a^b = \begin{bmatrix}
    R_a^b  & t_a^b \\
    0_{1\times 3} & 1
    \end{bmatrix}
\end{equation}

\noindent the expression for a point on the attackable surface in the camera reference frame is

\begin{equation}
    p^C = T_W^C T_S^W p^S
\end{equation}
\noindent where $T_W^C$ is the world-to-camera rototranslation, and $T_S^W$ is the surface-to-world rototranslation.

The resulting point can be projected with a pinhole camera model, which is the one used by CARLA RGB camera sensor. The projection, which is expressed in pixels, and identify the position of the point on the image, can be obtained as
\begin{equation}
    p_{pixels} = K p^C
\end{equation}
\noindent where $K$ is the intrinsic matrix of the CARLA RGB camera sensor. Its general form is
\begin{equation}
    K= \begin{bmatrix}
    f & 0 & c_x \\
    0 & f & c_y \\
    0 & 0 & 1
    \end{bmatrix}
\end{equation}
\noindent where $f$ is the focal, and $(c_x, c_y)$ is the center of the image expressed in pixels (and still in homogeneous coordinate). For the CARLA RGB camera sensor, these parameters are easy to compute: the focal $f=\frac{w}{\tan FOV / 2}$ (where $FOV$ is the field of view in radians - $\pi/2$ by default - and $w$ the image width), and the center of the image is simply $(w/2, h/2)$ (where $h$ is the image height). 

Then, to apply the patch, it is sufficient to compute a warping transformation, which maps the patch starting corners to the destination points on the image, computed as described above. The estimation of the warping transformation is done with the PyTorch-based library Kornia \cite{2019arXiv191002190R}. 

The transformation is then applied to the patch, which is correctly applied to the attackable surface.

\section{CARLA environmental settings and finetuning} \label{s:carla}
The fine-tuning of the models on the CARLA dataset was not an easy task: the images generated with CARLA sample a completely different distribution than Cityscapes. This justifies the limited performance on CARLA images of state-of-the-art models pre-trained on Cityscapes% (summarized in Table \ref{table:pretrained_acc})
: despite being built on Unreal Engine, CARLA lacks the photo-realism of that the modern graphic engines make available, often for free. 

\begin{comment}
\begin{table}[]
\centering
\resizebox{8.45cm}{!}{%
\begin{tabular}{|c|c|c|}
\hline
model        & \multicolumn{2}{c|}{mIoU / mAcc} \\ \hline
   & cityscapes      & CARLA (val - scene1 - scene2 -scene3)
\\ \hline
ICNet   & 0.00 ~/~0.00       & 0.00~/~0.00 - 0.00~/~0.00 - 0.00~/~0.00 - 0.00~/~0.00 \\ \hline
BiseNet & 0.69~/~0.78       & 0.00~/~0.00 - 0.00~/~0.00 - 0.00~/~0.00 - 0.00~/~0.00      \\ \hline
DDRNet  & 0.78~/~0.85       & 0.00~/~0.00 - 0.00~/~0.00 - 0.00~/~0.00 - 0.00~/~0.00      \\ \hline
PSPNet  & 0.00~/~0.00       & 0.00~/~0.00 - 0.00~/~0.00 - 0.00~/~0.00 - 0.00~/~0.00      \\ \hline
PSANet  & 0.00~/~0.00       & 0.00~/~0.00 - 0.00~/~0.00 - 0.00~/~0.00 - 0.00~/~0.00      \\ \hline
\end{tabular}
}
 \vspace{-1em}
\caption{mIoU and mAcc of the pretrained models used throughout the paper on Cityscapes and our CARLA dataset.}
\label{table:app_pretrained_acc}
\vspace{-1.5em}
\end{table}
\end{comment}

The particular distribution of CARLA-generated images poses a series of challenges, each of which was addressed:
\begin{itemize}
    \item Some classes are very prone to overfitting, since a large fraction of the total pixels of each image belongs to the classes road, sidewalk (that makes up a vast portion of the image), sky, and vegetation in some settings. Since the pre-trained versions of the networks already had good performance on those classes, during the fine-tuning a weight of 0.01 was assigned to the loss corresponding to these classes. This workaround solves the overfitting problem.
    \item The distribution is not ``real-world", but digital, in the sense that it lacks the typical imperfections in the meshes composing the scene. Additionally, no camera noise is considered during acquisition. This was accounted for by adding noise during fine-tuning
    \item The weather conditions heavily affect the appearance of the images, making the distribution change drastically. In order to avoid re-training from scratch, the choice fell on keeping the weather condition fixed as cloudy, as in the Cityscapes dataset.
\end{itemize}

INSERT PER-CLASS IOU and comment on the low mIOU.

\section{Additional details on experimental settings}

\subsection{Models description} \label{s:models}
To provide fair experiments we used pretrained models published by the authors. Each network structure was imported into our repository keeping the original mean and std variation required by all the pretrained version.
As introduced in \ref{s:exp}, the first three models are designed for run-time semantic segmentation, while the last two are more expensive in terms of memory footprint and execution time, but needed to provide a comparative analysis with the work of Nakka et. al. \cite{nakka_indirect_2019}. 

\paragraph{DDRNet}
We used the DDRNet23Slim version provided by the author \cite{ddrnet_paper}\footnote{https://github.com/ydhongHIT/DDRNet} that has shown to be one of fastest network in the state of the art of run-time SS.

\paragraph{BiseNet}
We used the original Pytorch implementation~\cite{bisenet_paper}
\footnote{https://github.com/ycszen/TorchSeg} with its pretrained weights. The applied version uses an Xception39 model \cite{xception}  as backbone.  

\paragraph{ICNet}
The original pretrained model \footnote{https://github.com/hszhao/ICNet} is provided by the authors~\cite{icnet_paper}, that was trained among  the Cityscapes train set for 30K epochs using the Caffe framework\cite{caffe}. 

\paragraph{PSPNet}
Also for this model we imported the original Caffe pretrained version provided by~\cite{pspnet_paper}\footnote{https://github.com/hszhao/PSPNet} that uses a RESNet101 \cite{2015arXiv151203385H} as backbone for feature extraction. 

\begin{comment}
\paragraph{PSANet}
Differently by \cite{nakka_indirect_2019}, we did not use directly the pretrained Pytorch version provided by the authors~\cite{psanet_paper} \footnote{https://github.com/hszhao/PSANet}, since it was trained with a different image-size that could produce unfair results during the experimental part. Indeed, we performed a finetuning of the model for 30 epochs on the Cityscapes train set starting from an already pretrained ResNet50 \cite{2015arXiv151203385H} backbone (available in the same repository). For this training we used the Adam optimizer with learning rate X and all the others default settings, finally the original pixel-wise cross entropy as loss function.
\end{comment}

\section{Additional results}\label{s:add_res}

\subsection{Robustness analysis for digital patch}\label{s:add_res_robust_digital}

\subsection{Digital patches}\label{s:add_res_digital}

COMMENT

\begin{figure*}[!t]
\centering
\makebox[\columnwidth]{\includegraphics[scale=0.80]{img/appendix/eot_test/appendix_pached_images.png}}
        \vspace{-1em}
\caption{First image represent a patched image with a random patch, while the others are adversarial patches ($200 \times 400$) obtained with Bisenet, DDRNet and ICNet, and PSPNet respectively.}
\label{fig:app_digital_gamma_ablation}
\end{figure*}

\begin{figure*}[!t]
     \centering
     \begin{subfigure}{0.33\textwidth}
         \centering
         \includegraphics[width=0.95\textwidth]{img/appendix/eot_test/appendix_res_ddrnet.png}
         \caption{}
         \label{fig:app_digital_exps_a}
     \end{subfigure}
     \begin{subfigure}{0.33\textwidth}
         \centering
         \includegraphics[width=0.95\textwidth]{img/appendix/eot_test/appendix_res_icnet.png}
         \caption{}
         \label{fig:app_digital_exps_b}
     \end{subfigure}
     \begin{subfigure}{0.33\textwidth}
         \centering
         \includegraphics[width=0.95\textwidth]{img/appendix/eot_test/appendix_res_pspnet.png}
         \caption{}
         \label{fig:app_digital_exps_c}
     \end{subfigure}
        \vspace{-1em}
        \caption{Semantic segmentations obtained from DDRNet (a), ICNet (b), PSPNet (c). For each block, the first column represents SS obtained from images patched with random patches ($200 \times 400$), while the second column refers to EoT-based patches.}
        \label{fig:app_digital_exps}
\end{figure*}

\begin{figure*}[!t]
\centering
     \begin{subfigure}{\textwidth}
         \centering
         \includegraphics[width=\textwidth]{img/appendix/eot_test/pspnet_hist_cityscapes.png}
         \caption{}
         \label{fig:app_digital_exps_b}
     \end{subfigure}
     \begin{subfigure}{\textwidth}
         \centering
         \includegraphics[width=\textwidth]{img/appendix/eot_test/bisenet_hist_cityscapes.png}
         \caption{}
         \label{fig:app_digital_exps_c}
     \end{subfigure}
        \vspace{-1em}
        \caption{Per class mIoU comparison on Cityscapes. Each bar shows the mIoU, computed on the valdiation, associated to a certain class. The results provide a comparison with no patch applied into the images (original dataset), random patches, EoT-based and no-EoT-based patches. The reference networks were PSPNet (a) and BiseNet (b).}
        \label{fig:app_digital_exps}
\end{figure*}

\subsection{Loss function ablation for scene-specific attack}
Figure \ref{fig:specific_gamma_ablation} the same study performed on the loss function for the EOT-based attack. The performance of the attack is reported for the three scenes. Clearly, the extension of the cross-entropy outperforms the classical cross-entropy for almost all value of $\gamma$.

\begin{figure*}[!t]
\centering
\makebox[\columnwidth]{\includegraphics[scale=0.38]{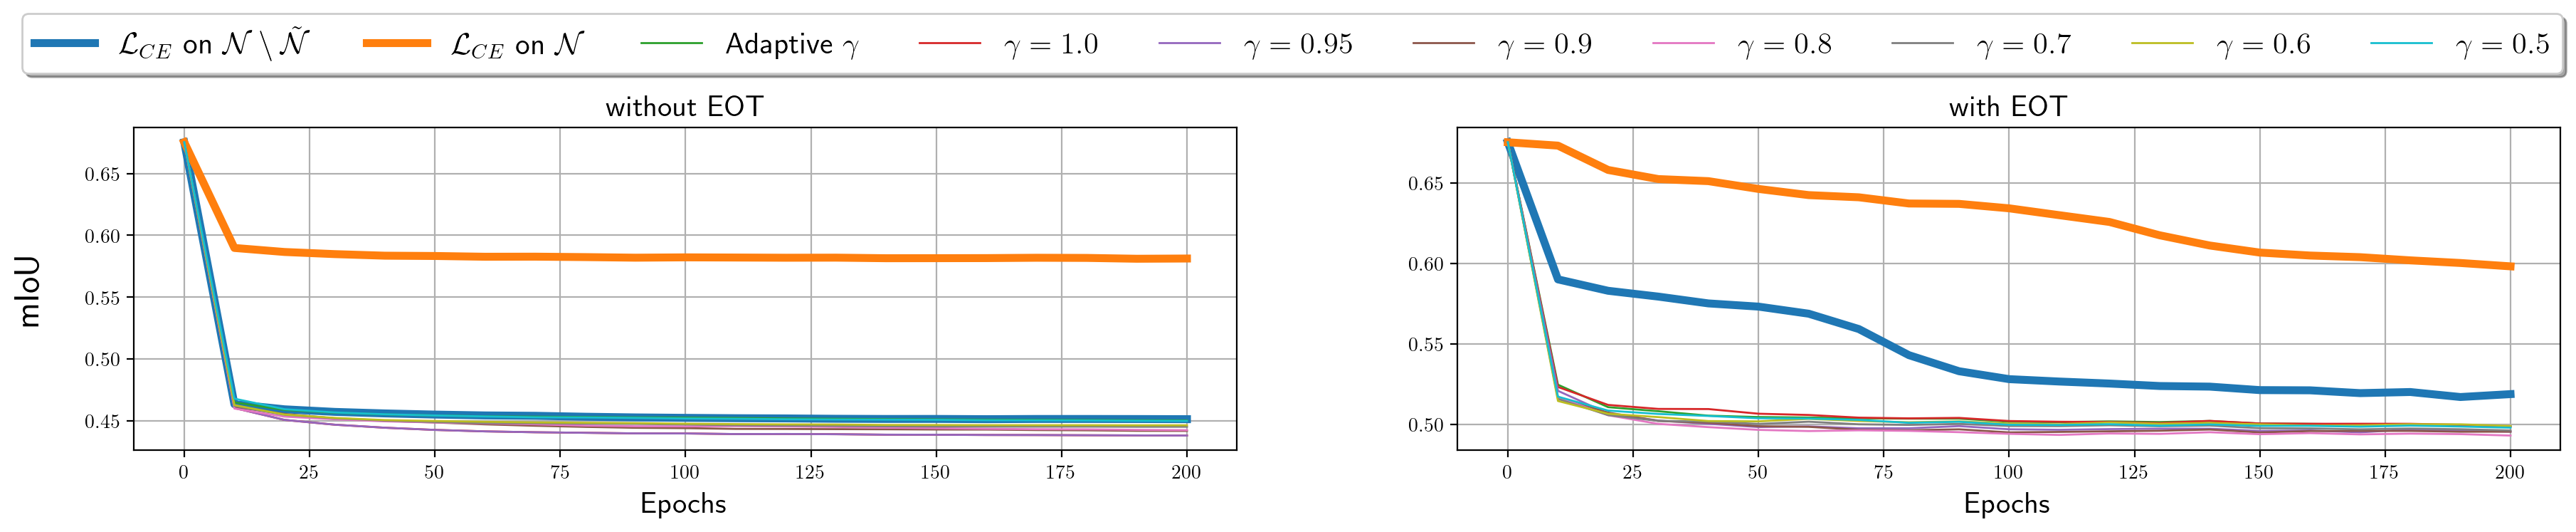}}
\caption{Adversarial patch ($150 \times 300$) optimizations with different loss functions.}
\label{fig:app_specific_gamma_ablation}
\end{figure*}

\subsection{Black-box transfer across models}
This section summarizes the cross-model black-box evaluation in Table \ref{table:black_box_carla}.

\begin{table*}[!t]
\centering
\small
\begin{tabular}{|c|c|l|c|l|c|l|c|l|}
\hline
Model   & \multicolumn{6}{c|}{\begin{tabular}[c]{@{}c@{}}mIoU  |  mAcc \quad(scene-specific /EOT)\end{tabular}}         \\ \hline
\begin{tabular}{@{}c@{}} Evaluated on $\rightarrow$ \\ Optimized on $\downarrow$ \end{tabular}   & \multicolumn{2}{c|}{\begin{tabular}[c]{@{}c@{}}ICNet\end{tabular}}  & \multicolumn{2}{c|}{\begin{tabular}[c]{@{}c@{}}BiseNet\end{tabular}} & \multicolumn{2}{c|}{\begin{tabular}[c]{@{}c@{}}DDRNet\end{tabular}}   \\ \hline
%        & \multicolumn{2}{c|}{Scene1}          & \multicolumn{2}{c|}{Scene2}          & \multicolumn{2}{c|}{Scene3}          \\ \hline
ICNet   & \begin{tabular}{@{}c@{}} 0.48 /0.49 \\ 0.61 /0.61 \\ 0.59 /0.59 \end{tabular} & \begin{tabular}{@{}c@{}} 0.54 /0.56 \\ 0.73 /0.73 \\ 0.74 /0.73 \end{tabular} & \begin{tabular}{@{}c@{}} 0.44 /0.44 \\ 0.60 /0.60 \\ 0.47 /0.47 \end{tabular} & \begin{tabular}{@{}c@{}} 0.61 /0.60 \\ 0.75 /0.76 \\ 0.74 /0.74 \end{tabular} & \begin{tabular}{@{}c@{}} 0.50 /0.51 \\ 0.62 /0.61 \\ 0.65 /0.65 \end{tabular} & \begin{tabular}{@{}c@{}} 0.69 /0.70 \\ 0.75 /0.75 \\ 0.78 /0.78 \end{tabular} \\ \hline %& \begin{tabular}{@{}c@{}} nd \\  nd\\ nd \end{tabular} & \begin{tabular}{@{}c@{}} nd  \\ nd \\ nd \end{tabular} \\ \hline
BiseNet   & \begin{tabular}{@{}c@{}} 0.50 /0.51 \\ 0.63 /0.63 \\ 0.63 /0.63 \end{tabular} & \begin{tabular}{@{}c@{}} 0.60 /0.60 \\ 0.73 /0.73 \\ 0.75 /0.75 \end{tabular} & \begin{tabular}{@{}c@{}} 0.31 /0.36 \\ 0.58 /0.58 \\ 0.45 /0.46 \end{tabular} & \begin{tabular}{@{}c@{}} 0.49 /0.55 \\ 0.74 /0.74 \\ 0.73 /0.73 \end{tabular} & \begin{tabular}{@{}c@{}} 0.50 /0.50 \\ 0.62 /0.62 \\ 0.65 /0.65 \end{tabular} & \begin{tabular}{@{}c@{}} 0.69 /0.70 \\ 0.75 /0.75 \\ 0.78 /0.78 \end{tabular} \\ \hline % & \begin{tabular}{@{}c@{}} nd \\  nd\\ nd \end{tabular} & \begin{tabular}{@{}c@{}} nd  \\ nd \\ nd \end{tabular} \\ \hline
DDRNet   & \begin{tabular}{@{}c@{}} 0.51 /0.51 \\ 0.63 /0.63 \\ 0.63 /0.63 \end{tabular} & \begin{tabular}{@{}c@{}} 0.60 /0.60 \\ 0.73 /0.73 \\ 0.75 /0.75 \end{tabular} & \begin{tabular}{@{}c@{}} 0.44 /0.44 \\ 0.60 /0.60 \\ 0.47 /0.47 \end{tabular} & \begin{tabular}{@{}c@{}} 0.60 /0.60 \\ 0.75 /0.76 \\ 0.74 /0.74 \end{tabular} & \begin{tabular}{@{}c@{}} 0.46 /0.46 \\ 0.49 /0.52 \\ 0.59 /0.58 \end{tabular} & \begin{tabular}{@{}c@{}} 0.69 /0.69 \\ 0.66 /0.71 \\ 0.76 /0.76 \end{tabular} \\ \hline %& \begin{tabular}{@{}c@{}} nd \\  nd\\ nd \end{tabular} & \begin{tabular}{@{}c@{}} nd  \\ nd \\ nd \end{tabular} \\ \hline
%PSPNet   & \begin{tabular}{@{}c@{}} 0.48 /0.00 \\ 0.48 /0.00 \\ 0.48 /0.00 \end{tabular} & \begin{tabular}{@{}c@{}} 0.48 /0.00 \\ 0.48 /0.00 \\ 0.48 /0.00 \end{tabular} & \begin{tabular}{@{}c@{}} 0.48 /0.00 \\ 0.48 /0.00 \\ 0.48 /0.00 \end{tabular} & \begin{tabular}{@{}c@{}} 0.48 /0.00 \\ 0.48 /0.00 \\ 0.48 /0.00 \end{tabular} & \begin{tabular}{@{}c@{}} 0.48 /0.00 \\ 0.48 /0.00 \\ 0.48 /0.00 \end{tabular} & \begin{tabular}{@{}c@{}} 0.48 /0.00 \\ 0.48 /0.00 \\ 0.48 /0.00 \end{tabular} & \begin{tabular}{@{}c@{}} nd \\  nd\\ nd \end{tabular} & \begin{tabular}{@{}c@{}} nd  \\ nd \\ nd \end{tabular} \\ \hline
%PSANet   & \begin{tabular}{@{}c@{}} 0.48 /0.00 \\ 0.48 /0.00 \\ 0.48 /0.00 \end{tabular} & \begin{tabular}{@{}c@{}} 0.48 /0.00 \\ 0.48 /0.00 \\ 0.48 /0.00 \end{tabular} & \begin{tabular}{@{}c@{}} 0.48 /0.00 \\ 0.48 /0.00 \\ 0.48 /0.00 \end{tabular} & \begin{tabular}{@{}c@{}} 0.48 /0.00 \\ 0.48 /0.00 \\ 0.48 /0.00 \end{tabular} & \begin{tabular}{@{}c@{}} 0.48 /0.00 \\ 0.48 /0.00 \\ 0.48 /0.00 \end{tabular} & \begin{tabular}{@{}c@{}} 0.48 /0.00 \\ 0.48 /0.00 \\ 0.48 /0.00 \end{tabular} \\ \hline
\end{tabular}
\caption{Black-box transferability across models in terms of mIOU and mAcc. The results are showed for both the EOT-based and the scene-specific, for the three scenes of the CARLA datasets.}
\label{table:black_box_carla}
\end{table*}

\begin{table*}[!t]
\centering
\small
\begin{tabular}{|c|c|c|c|c|c|c|c|c|}
\hline
Model   & \multicolumn{8}{c|}{mIoU - mAcc}                                                                                                                                                          \\ \hline
\begin{tabular}{@{}c@{}} Evaluated on $\rightarrow$ \\ Optimized on $\downarrow$ \end{tabular}      & \multicolumn{2}{c|}{\begin{tabular}[c]{@{}c@{}}ICNet\end{tabular}} & \multicolumn{2}{c|}{\begin{tabular}[c]{@{}c@{}}BiseNet\end{tabular}} & \multicolumn{2}{c|}{\begin{tabular}[c]{@{}c@{}}DDRNet\end{tabular}} & \multicolumn{2}{c|}{\begin{tabular}[c]{@{}c@{}}PSPNet\end{tabular}} \\ \hline
ICNet   & 0.50                 & 0.61                 & 0.54                  & 0.69                  & 0.62                  & 0.79                 & 0.68                  & 0.76                 \\ \hline
BiseNet & 0.62                 & 0.71                 & 0.29                  & 0.43                  & 0.62                  & 0.79                 & 0.69                  & 0.77                 \\ \hline
DDRNet  & 0.65                 & 0.75                 & 0.56                  & 0.68                  & 0.59                  & 0.69                 & 0.67                  & 0.77                 \\ \hline
PSPNet  & 0.65                 & 0.78                 & 0.58                  & 0.70                  & 0.67                  & 0.80                 & 0.23                  & 0.30                 \\ \hline
\end{tabular}
\caption{Black-box transferability on the Cityscapes dataset across models in terms of mIOU and mAcc. The results are showed for EOT-based patches.}
\label{table:black_box_cityscapes}
\end{table*}

\begin{figure*}[!t]
\centering
\makebox[\columnwidth]{\includegraphics[scale=0.80]{img/appendix/carla_results/appendix_pached_images_carla.png}}
        \vspace{-1em}
\caption{First image represent a patched image with a random patch, while the others are adversarial patches ($200 \times 400$) obtained with Bisenet, DDRNet and ICNet,respectively.}
\label{fig:app_digital_gamma_ablation}
\end{figure*}

\begin{figure*}[!t]
     \centering
     \begin{subfigure}{0.48\textwidth}
         \centering
         \includegraphics[width=0.95\textwidth]{img/appendix/carla_results/appendix_res_carla_bisenet.png}
         \caption{}
         \label{fig:app_digital_exps_a}
     \end{subfigure}
     \begin{subfigure}{0.48\textwidth}
         \centering
         \includegraphics[width=0.95\textwidth]{img/appendix/carla_results/appendix_res_carla_icnet.png}
         \caption{}
         \label{fig:app_digital_exps_b}
     \end{subfigure}
        \vspace{-1em}
        \caption{Semantic segmentations obtained from BiseNet (a) and ICNet (b) on CARLA Scene-1. For each block, the first column is the SS obtained from images patched with random patches, the second represents the patched image with the patch optimized with the scene-specific attack, and finally, the third column is its predicted SS.}
        \label{fig:app_digital_exps}
\end{figure*}

\begin{figure*}[!t]
\centering
     \begin{subfigure}{\textwidth}
         \centering
         \includegraphics[width=\textwidth]{img/appendix/carla_results/appendix_hist_bisenet_carla.png}
         \caption{}
         \label{fig:app_digital_exps_b}
     \end{subfigure}
     \begin{subfigure}{\textwidth}
         \centering
         \includegraphics[width=\textwidth]{img/appendix/carla_results/appendix_hist_ddrnet_carla.png}
         \caption{}
         \label{fig:app_digital_exps_c}
     \end{subfigure}
        \vspace{-1em}
        \caption{Per class mIoU comparison on Carla. Each bar shows the mIoU corresponding to a certain class on the proposed Carla dataset (we kept the same cityscapes classes) for Scene-1 (a) and Scene-2 (b), both meausered with their validation sets. The results show a comparison with random patch, EoT-based optimization and the proposed scene-specific on Bisenet (a) and DDRNet (b). All the patches were imported directly in Carla in order to provide a fair attack evaluation, as close as possible to a real world scenario.}
        \label{fig:app_digital_exps}
\end{figure*}

\begin{figure*}[!t]
     \centering
     \begin{subfigure}{0.33\textwidth}
         \centering
         \includegraphics[width=0.9\textwidth]{img/appendix/patches/bisenet_02.png}
         \caption{}
     \end{subfigure}
     \begin{subfigure}{0.33\textwidth}
         \centering
         \includegraphics[width=0.9\textwidth]{img/appendix/patches/icnet_02.png}
         \caption{}
     \end{subfigure}
     \begin{subfigure}{0.33\textwidth}
         \centering
         \includegraphics[width=0.9\textwidth]{img/appendix/patches/ddrnet_02.png}
         \caption{}
     \end{subfigure}
     \begin{subfigure}{0.33\textwidth}
         \centering
         \includegraphics[width=0.9\textwidth]{img/appendix/patches/rw_patch_icnet.png}
         \caption{}
     \end{subfigure}
     \begin{subfigure}{0.33\textwidth}
         \centering
         \includegraphics[width=0.9\textwidth]{img/appendix/patches/rw_patch_ddrnet.png}
         \caption{}
     \end{subfigure}
     \begin{subfigure}{0.33\textwidth}
         \centering
         \includegraphics[width=0.9\textwidth]{img/appendix/patches/cityscapes_pspnet_400.png}
         \caption{}
     \end{subfigure}
    \vspace{-1em}
    \caption{Patches obtained using specific attack on CARLA-scene 1 with Bisenet (a), ICNet (b), DDRNet (c), while (d) and (e) are patches optimized using a digital EoT on the Pisa-scapes dataset on ICNet and DDRNet, respectively. Finally, (f) is a patch optimized using again a digital EoT on Cityscapes with PSPNet.}
    \label{fig:app_digital_exps}
\end{figure*}

\begin{figure*}[!t]
     \centering
     \begin{subfigure}{0.48\textwidth}
         \centering
         \includegraphics[width=0.95\textwidth]{img/appendix/real-world/appendix_rw_rand.png}
         \caption{}
         \label{fig:app_digital_exps_a}
     \end{subfigure}
     \begin{subfigure}{0.48\textwidth}
         \centering
         \includegraphics[width=0.95\textwidth]{img/appendix/real-world/appendix_rw_adv.png}
         \caption{}
         \label{fig:app_digital_exps_b}
     \end{subfigure}
        \vspace{-1em}
        \caption{Real-world adversarial patch effects compute on our Pisa-scapes. images in (a) contain a printed random patch, while in (b) a printed adversarial patch was used. It has been optimized with a digital EoT on ICNet using a secondary set of the same scene. For all the sampled images the corresponding semantic segmentation is placed on the right.}
        \label{fig:app_digital_exps}
\end{figure*}
